# Supplementary material for: Probabilistic Stability Guarantees for Feature Attributions
Source: arXiv:2504.13787 source file (2025-08-07)
Supplement: Supplementary file 1 [file old_appendix_dump.tex]

\newpage


\section{Proofs and Deletion \bise}

\subsection{Insertion \bise Bounds Proof Details}
In this section, we prove Lemma~\ref{bise_ins_bounds}, which is a direct application of Boolean set influences to the \bise metric. 
Let $f: \mathbb{R}^n \to \R^c$ be a model, and let $g$ be the boolean function as defined in Section~\ref{sec:bise}.

Suppose $v_k = \textbf{Inf}_f (S_k) / 2$ for the set of top $k$ features $S_k \subseteq [n]$ and true insertion BISE $\textbf{Ins\bise}_f (A) = AUC[V]$ where $V$ is the sequence of of values $v_k$ where $k = 1$ to $n$.  

Then by Lemma 2.2.3 of \citet{levi2020tolerant}, if $\epsilon$ is small enough, then the approximate influence calculation in Algorithm \ref{alg:approx_influence} results in the following bounds on each $v_k$:
$$\frac{1-\gamma}{2} \cdot  \textbf{Inf}_f(S_k) \leq v_k \leq \frac{1+\gamma}{2}  \cdot \textbf{Inf}_f (S_k) $$
Plugging this into the definition of the Insertion \bise score completes the proof. 

% \begin{theorem}
%     % \label{bise_ins_bounds}
%     (Insertion \bise \ estimation bounds) Let $f: \mathbb{R}^n \to \R^c$ be a model, and let $g$ be the boolean function as defined in Section~\ref{sec:bise}. Then by Lemma 2.2.3 of \citet{levi2020tolerant}, the influence calculation in Algorithm \ref{alg:influence_ins_score}
%     %) that receives an oracle access to $f$, feature attributions $A \in \mathbb{R}^n$ for input $x \in \mathbb{R}^n$, and $\gamma, \delta, \epsilon \in (0,1)$, uses $m = O(\frac{\log(1/\delta)}{\epsilon \cdot \gamma^2})$ queries to $f$, and 
%     satisfies the following with probability at least $1-\delta$:\footnote{Note that we are using the trapezoidal rule to calculate Area Under the Curve (AUC). This accounts for $\frac{1}{n}$ factor in the bounds.} 

%     Suppose $v_k = \textbf{Inf}_f (S_k) / 2$ for the set of top $k$ features $S_k \subseteq [n]$ and true insertion BISE $\textbf{Ins\bise}_f (A) = AUC[V]$ where $V$ is the sequence of of values $v_k$ where $k = 1$ to $n$. 

    %  \begin{enumerate}
    %     \item If $v_k = \textbf{Inf}_f (S_k) / 2 \geq \epsilon$, then the algorithm outputs an estimate $\widetilde{\textbf{Ins\bise}}_f (A)$ such that 
    %     $$ \frac{1-\gamma}{2n} \cdot \sum_{k}  \textbf{Inf}_f(S_k) \leq \widetilde{\textbf{Ins\bise}}_f (A) \leq \frac{1+\gamma}{2n}  \cdot \sum_{k} \textbf{Inf}_f (S_k) $$
        
    %     \item If $v_k = \textbf{Inf}_f (S_k) / 2 < \epsilon$ for $S_k$, then the algorithm outputs estimate $\widetilde{\textbf{Ins\bise}}_f (A)$ such that 
    %     $$ \widetilde{\textbf{Ins\bise}}_f (A) \leq \frac{1_+ \gamma}{2n}  \cdot \sum_{k} \textbf{Inf}_f (S_k) < \frac{(1 + \gamma)\cdot  \epsilon}{2} $$
    % \end{enumerate}
    % \begin{enumerate}
    %     \item If $v_k = \textbf{Inf}_f (S_k) \geq \epsilon$ for $S_k$ and true insertion BISE \textbf{Ins\bise}_f (A) = AUC[V]$ where $V$ is the sequence of of values $v_k$ where $k = 1$ to $n$, then the algorithm outputs an estimate $\widetilde{\textbf{Ins\bise}}_f (A)$ such that 
    %     $$ \frac{1-\gamma}{n} \cdot \sum_{k}  \textbf{Inf}_f(S_k) \leq \widetilde{\textbf{Ins\bise}}_f (A) \leq \frac{1+\gamma}{n}  \cdot \sum_{k} \textbf{Inf}_f (S_k) $$
        
    %     \item If $v_k = \textbf{Inf}_f (S_k) < \epsilon$ for $S_k$ and $\textbf{Ins\bise}_f (A) = AUC[V]$ where $V$ is the sequence of of values $v_k$ where $k = 1$ to $n$, then the algorithm outputs estimate $\widetilde{\textbf{Ins\bise}}_f (A)$ such that 
    %     $$ \widetilde{\textbf{Ins\bise}}_f (A) \leq \frac{1_+ \gamma}{n}  \cdot \sum_{k} \textbf{Inf}_f (S_k) < (1 + \gamma)\cdot  \epsilon $$
    % \end{enumerate}
% \end{theorem}

\subsection{Deletion \bise}
\label{bise_deletion}


\begin{definition} (Deletion BISE) We follow a modified version of the general framework presented in Subsection \ref{general_framework}. Suppose we are given a feature attribution $A \in \mathbb{R}^n$ for input $x \in \mathbb{R}^n$. Assume we also have a model $f: \mathbb{R}^n \to \R^c$, where $P = [0,1]^c$, which means model $f$ returns the class with the highest probability which we take to be the predicted class.

    Let the scoring function be $\phi (f, x, \alpha_k) = \textbf{Inf}_f (\bar{S}_k) / 2$,
    where $S_k \subseteq [n]$ is the set of top $k$ features specified by $\alpha_k$ and $\bar{S}_k$ is the complement set of $S_k$, i.e. $\bar{S}_k = [n] - S_k$. 
    \\
    \footnote{Unlike the original formulation presented in \citep{levi2020tolerant} and reproduced in Definition \ref{def:Set influence}, we divide the influence by a factor of 2 so that the scoring function has range $[0,1]$.}

    Then, the \textbf{Deletion \bise} of the feature attribution $A$ is defined as:
    \begin{align*}
        \textbf{DelBISE} (A)
        &= \text{AUC} [ \phi(f, x, \alpha_1), \ldots, \phi(f, x, \alpha_k), \ldots, \\
        &\quad\quad\quad\;  \phi(f, x, \alpha_n)] \\
        &= \text{AUC} [ \textbf{Inf}_f (\bar{S}_1)/2, \ldots, \textbf{Inf}_f (\bar{S}_k)/2, \ldots, \\
        &\quad\quad\quad\; \textbf{Inf}_f (\bar{S}_n)/2]
    \end{align*}
\end{definition} 

In practice, we find the estimate Deletion BISE, $\widetilde{\textbf{Del\bise}}_f (A)$, by taking the scoring function to be $\phi (f, x, \alpha_k) = \widetilde{\textbf{Inf}}_f (\bar{S}_k) / 2$, where each influence is approximated as specified in Algorithm \ref{alg:approx_influence}. As the Deletion \bise only changes the order in which features are considered along the AUC curve, the proof for the certified bounds for deletion \bise is exactly the same as for insertion. 

% \begin{algorithm} [ht!]
% \caption{Deletion \bise ($A, \epsilon, \gamma, \delta$)}\label{alg:influence_del_score}
% \begin{algorithmic}
%     \State We follow a modified version of the general framework presented in Subsection \ref{general_framework}. 

%     \State Suppose we are given a feature attribution $A \in \mathbb{R}^n$ for input $x \in \mathbb{R}^n$. \State Assume we also have a model $f: \mathbb{R}^n \to \R^c$, where $P = [0,1]^c$, which means model $f$ returns the class with the highest probability which we take to be the predicted class.\\

%     \State Let the scoring function be $\phi (f, x, \alpha_k) = \textbf{Inf}_f (\bar{S}_k) / 2$,
%     where $S_k \subseteq [n]$ is the set of top $k$ features specified by $\alpha_k$ and $\bar{S}_k$ is the complement set of $S_k$, i.e. $\bar{S}_k = [n] - S_k$. 
%     \\
%     \Comment{Unlike the original formulation presented in \citep{levi2020tolerant} and reproduced in Definition \ref{def:Set influence}, we divide the influence by a factor of 2 so that the scoring function has range $[0,1]$.}

%     \State Then, the \textbf{Deletion \bise} of the feature attribution $A$ is defined as:
%     \begin{align*}
%         \textbf{DelBISE} (A)
%         &= \text{AUC} [ \phi(f, x, \alpha_1), \ldots, \phi(f, x, \alpha_k), \ldots, \phi(f, x, \alpha_n)] \\
%         &= \text{AUC} [ \textbf{Inf}_f (\bar{S}_1)/2, \ldots, \textbf{Inf}_f (\bar{S}_k)/2, \ldots, \textbf{Inf}_f (\bar{S}_n)/2]
%     \end{align*}
%     \\
%     \Comment{In practice, we find the estimate Deletion BISE, $\widetilde{\textbf{Del\bise}}_f (A)$, by taking the scoring function to be $\phi (f, x, \alpha_k) = \widetilde{\textbf{Inf}}_f (\bar{S}_k) / 2$,
%     where each influence is approximated as specified in Algorithm \ref{alg:approx_influence}. }
% \end{algorithmic}
% \end{algorithm}


% \subsection{\bise \ Deletion Score}
% \begin{algorithm} %[t]
% \caption{Influence Deletion Score ($A, \epsilon, \gamma, \delta$)}\label{alg:influence_del_score}
% \begin{algorithmic}
%     \State We follow a modified version of the general framework presented in Subsection \ref{general_framework}. 
%     \\ 
%     \State Suppose we are given a feature attribution $A \in \mathbb{R}^n$ for input $x \in \mathbb{R}^d$. 
%     \State Assume we also have a model $f: \mathbb{R}^d \to \R^c$, where $P = [0,1]^c$, which means model $f$ returns the class with the highest probability which we take to be the predicted class. \\
%     \For{$k$ = 1 to $n$}
%     \State 1. Let $a_{(k)}$ denote the $k^{th}$ order statistic.
%     \State 2. Construct the mask $\alpha_k \in \{0,1\}^n$ such that all values in $A$ greater than or equal to $A_{(n - k)}$ are marked as 1 in $\alpha_k$ and 0 otherwise. 
%     \State 3. Translate $\alpha_k$ to its corresponding set of top $k$ features and call this set $S_k$, where $S_k \subseteq [n]$.  
%     \State 4. Let $\bar{S}_k$ be the complement of $S_k$, namely $\bar{S}_k = [n] - S_k$.
%     \State 5. Set $v_k$ = $\widetilde{\textbf{Inf}}_f (\bar{S}_k) / 2$.
%     \Comment{Unlike the original formulation presented in \citep{levi2020tolerant} and reproduced in Algorithm \ref{alg:approx_influence}, we divide the approximate influence by a factor of 2 so that value $v_k$ has range $[0,1]$.}
%     \EndFor \\

%     \State Let $V$ be the sequence of values $v_k$, where $k = 1$ to $n$.
%     \State Then, the \textbf{influence deletion score} is defined as:
%     $$InfDelScore(A) =  AUC(V)$$ 
   
%     % sequence of values $f(x \odot \alpha_k)$ 
   
% \end{algorithmic}
% \end{algorithm}


% \subsection{Deletion \bise Bounds Proof Details}

% \begin{theorem}
%     \label{bise_del_bounds}
%     (Deletion \bise bounds with estimation) Let $f: \mathbb{R}^n \to \R^c$ be a model where $P = [0,1]^c$, which means model $f$ returns the class with the highest probability which we take to be the predicted class. Given an oracle access to $f$, feature attributions $A \in \mathbb{R}^n$ for input $x \in \mathbb{R}^n$, and $\gamma, \delta, \epsilon \in (0,1)$, $m = O(\frac{\log(1/\delta)}{\epsilon \cdot \gamma^2})$ queries to $f$, we can say with probability at least $1-\delta$ that the true insertion \bise, $\textbf{Del\bise}_f (A)$, is bounded as follows:\footnote{Note that we are using the trapezoidal rule to calculate Area Under the Curve (AUC). This accounts for $\frac{1}{n}$ factor in the denominator.}

%     $$\frac{\widetilde{\textbf{Del\bise}}_f (A)}{1 + \gamma} \leq \textbf{Del\bise}_f (A) \leq \max \Bigl(\frac{\widetilde{\textbf{Del\bise}}_f (A)}{1- \gamma}, \frac{\epsilon}{2} \Bigl)$$

%     where $\widetilde{\textbf{Del\bise}}_f (A)$ is the estimate of insertion \bise.
% \end{theorem}

% \begin{theorem}
%     % \label{bise_del_bounds}
%     (Deletion \bise \ estimation bounds) Let $f: \mathbb{R}^n \to \R^c$ be a model where $P = [0,1]^c$, which means model $f$ returns the class with the highest probability which we take to be the predicted class. There exists an algorithm (namely, Algorithm \ref{alg:influence_ins_score}) that receives an oracle access to $f$, feature attributions $A \in \mathbb{R}^n$ for input $x \in \mathbb{R}^n$, and $\gamma, \delta, \epsilon \in (0,1)$, uses $m = O(\frac{\log(1/\delta)}{\epsilon \cdot \gamma^2})$ queries to $f$, and satisfies the following with probability at least $1-\delta$:\footnote{Note that we are using the trapezoidal rule to calculate Area Under the Curve (AUC). This accounts for $\frac{1}{n}$ factor in the bounds.} 

%         Suppose $v_k = \textbf{Inf}_f (\bar{S}_k) / 2$ for the set of top $k$ features $S_k \subseteq [n]$ and true deletion BISE $\textbf{Del\bise}_f (A) = AUC[V] = \frac{1}{2n} \sum_{k}  \textbf{Inf}_f(\bar{S}_k)$ where $V$ is the sequence of of values $v_k$ where $k = 1$ to $n$.
%     \begin{enumerate}
%         \item If $v_k = \textbf{Inf}_f (\bar{S}_k) / 2 \geq \epsilon$, then the algorithm outputs an estimate $\widetilde{\textbf{Del\bise}}_f (A)$ such that 
%         $$ \frac{1-\gamma}{2n} \cdot \sum_{k}  \textbf{Inf}_f(\bar{S}_k) \leq \widetilde{\textbf{Del\bise}}_f (A) \leq \frac{1+\gamma}{2n}  \cdot \sum_{k} \textbf{Inf}_f (\bar{S}_k) $$
        
%         \item If $v_k = \textbf{Inf}_f (\bar{S}_k) / 2 < \epsilon$, then the algorithm outputs estimate $\widetilde{\textbf{Del\bise}}_f (A)$ such that 
%         $$ \widetilde{\textbf{Del\bise}}_f (A) \leq \frac{1+ \gamma}{2n}  \cdot \sum_{k} \textbf{Inf}_f (\bar{S}_k) < \frac{(1 + \gamma)\cdot  \epsilon}{2} $$
%     \end{enumerate}

%     % \begin{enumerate}
%     %     \item If $v_k = \textbf{Inf}_f (\bar{S}_k) \geq \epsilon$ for the set of top $k$ features $S_k \subseteq [n]$ and true deletion BISE \textbf{Del\bise}_f (A) = AUC[V]$ where $V$ is the sequence of of values $v_k$ where $k = 1$ to $n$, then the algorithm outputs an estimate $\widetilde{\textbf{Del\bise}}_f (A)$ such that 
%     %     $$ \frac{1-\gamma}{n} \cdot \sum_{k}  \textbf{Inf}_f(\bar{S}_k) \leq \widetilde{\textbf{Del\bise}}_f (A) \leq \frac{1+\gamma}{n}  \cdot \sum_{k} \textbf{Inf}_f (\bar{S}_k) $$
        
%     %     \item If $v_k = \textbf{Inf}_f (\bar{S}_k) < \epsilon$ for the set of top $k$ features $S_k \subseteq [n]$ and $\textbf{Del\bise}_f (A) = AUC[V]$ where $V$ is the sequence of of values $v_k$ where $k = 1$ to $n$, then the algorithm outputs estimate $\widetilde{\textbf{Del\bise}}_f (A)$ such that 
%     %     $$ \widetilde{\textbf{Del\bise}}_f (A) \leq \frac{1_+ \gamma}{n}  \cdot \sum_{k} \textbf{Inf}_f (\bar{S}_k) < (1 + \gamma)\cdot  \epsilon $$
%     % \end{enumerate}
% \end{theorem}
\section{Experimental Setup}
\label{experimentalsetup}

\subsection{Computational Configuration}
All experiments were conducted on two server machines with 8 NVIDIA A100 GPU's and 8 NVIDIA A6000 GPU's.

\subsection{Masking of Features}
% \subsubsection{Features + Masking}
\label{masking}
For a given image in ImageNet1K, we group the 3 x 224 x 224 pixels comprising the image into patches of size 3 x 28 x 28, which we use as our features. This leaves us with $n = 64$ features for every image. For a given tweet text in TweetEval, we tokenize the tweet and use each resulting token as a single feature. Depending on the length of the original tweet, there were 6-82 features for a particular tweet.
%\footnote{See Appendix \ref{text_experiments} for more details on the text setting.} 
For images, we mask a feature by replacing it in the image with a zero. For text, to mask a token, we replace the token in the original tweet with the [MASK] token.

% \subsection{Human Evaluation}
% \label{app:human_eval}
% We perform the human evaluations on ImageNet.
% We take 1 image each from 5 random classes, totalling 5 images.
% For each image, for each metric, we have perturbation for window and swap.
% % We take 1 image each from 3 random classes, totalling 3 images.
% % For each image, for each metric, we have perturbation for window and swap.
% The four perturbations for each attribution we show to the evaluators have 4, 8, 12, and 16 features (patches) perturbed.
% % We randomly have two perturbed attributions to be the best perturbations while other two to be the worst.
% For each setting, we have two experiments, one alternates between best, worst, best, worst perturbations, and the other alternates between worst, best, worst, best perturabtion.
% Ideally, reliable metrics will have a smaller difference in scores for best and worst perturabtions for the same perturbation size, thus making it easier for humans to guess.
% For each task, we have three human evaluators.
% We compensate the evaluators with 0.05 dollers per task, estimated to be 7.5 dollars per hour with an average speed of 24 seconds per task.

% % \paragraph{Simulation.}
% Each evaluator is shown the original attribution along with the first four perturbations in order, along with scores of one metric (e.g. LeRF), and then asked to move the slider to guess the score for the last perturbed attribution.
% The scores are first flipped for Max Sensitivity, MoRF, Del. Test, Del. \bise to ensure that higher scores shown to the evaluators are better, to align with human intuitions.
% Then, the scores are also normalized to 0 $\sim$ 1 for each metric among scores for the whole dataset for that type of perturbation for that specific metric.
% These are performed to limit the bias humans can have with scores of different scales.
% The interface for simulation is shown in Figure~\ref{fig:human_eval_mturk}.

% In addition to the Pearson Correlation plot we show in Figure~\ref{fig:human-simulation-pearson} in the main paper for perturbation size 16, we also show it for size 8 in Figure~\ref{fig:human-simulation-pearson-3}. 
% When the perturbation size is small, \bise does not necessarily have the advantage of more human predictable.
% % Due to time constraint, this version we are showing takes 1 image each from 3 random classes, totalling 3 images.
% % We randomly have two perturbed attributions to be the best perturbations while other two to be the worst.
% We also show all the scatter plots for predicting perturbation size 16 and 8 in Figure~\ref{fig:scatter-human-simulation} and Figure~\ref{fig:scatter-human-simulation-3}.
% We can see that human can predict the scores well for Del. Test, MoRF and LeRF for perturbation size 8, but not for size 16. 
% This is because with a smaller perturbation size, the range of scores is still not a lot for the baselines, while it becomes a lot more when the perturbation size goes up.
% With a larger perturbation size, \bise shows the advantage with better human correlation in the simulation test.


% \paragraph{Satisfaction.} We also perform another human evaluation to ask humans about how much they trust the metric's scores.
% Instead of having the evaluator guess the score for the fifth perturbation, we show the scores for all five perturbations, and ask how much the person trusts that the score can represent how good the explanation is.
% The interface for satisfaction is shown in Figure~\ref{fig:human_eval_mturk_choices}.



% \begin{figure}
%     \centering
%     \includegraphics[width=\linewidth]{icml2025/figures/human_eval_mturk_choices/human_interface_choices1.png}
%     \includegraphics[width=\linewidth]{icml2025/figures/human_eval_mturk_choices/human_interface_choices2.png}
%     \caption{Human evaluation MTurk interface for satisfaction test.}
%     \label{fig:human_eval_mturk_choices}
% \end{figure}

\section{Additional ImageNet-1K Experiments}
\label{other_img}


\subsection{Ranking Stability Experiment Standard Deviations}

We use bootstrap (with replacement) to estimate standard deviations, and report the full results of the ranking stability experiments in Tables \ref{tab:stddev_window_imagenet} and \ref{tab:stddev_swap_imagenet} for window and swap perturbations respectively. We report $\pm 1$ SD for each setting.

\begin{table}
\centering
\fontsize{8.5}{10}\selectfont
    \begin{tabularx}{\linewidth}{c*{5}{X}}  
        \toprule
         & &   LIME  &   SHAP  &  IntGrad  &   Avg $\downarrow$ \\
        \midrule
    \multirow{ 3}{*}{Ins} & LeRF  &  10.2500 $\pm$ 2.7461 &  7.9699 $\pm$  1.0891   &  8.9399 $\pm$ 1.9300  &   9.0530    \\
    & Insertion Test  &  2.4400 $\pm$ 0.7735  &  3.8290 $\pm$ 1.3392  &  5.6599  $\pm$ 2.7492 &   3.9763   \\
    & \textbf{\bise}   &   0.9200 $\pm$ 0.5938   &   0.5699 $\pm$ 0.2549   &   1.7990  $\pm$ 0.5890  &   1.0963      \\
    \midrule
    \multirow{ 3}{*}{Del} & MoRF  &  11.1300 $\pm$  1.8408 &  10.6599 $\pm$ 2.0792  &  9.3900 $\pm$ 2.4747  &  10.3933    \\
    & Deletion Test  &  2.5199  $\pm$ 1.0848 &  4.7500 $\pm$ 1.2115  &  7.4099 $\pm$ 1.0245  &  4.8932     \\
    & \textbf{\bise}   &  0.5500 $\pm$ 0.2460    &  0.9300 $\pm$ 0.2864    &  1.7300 $\pm$ 0.7061    &  1.0700        \\
        \bottomrule
    \end{tabularx}
    % \vskip{-0.1}  
    \caption{Mean rank difference percentages with $\pm 1$ SD across Window perturbations (sz = 12) for insertion and deletion metrics; ImageNet-1K. }\label{tab:stddev_window_imagenet}
\end{table}


  



\begin{table}
\centering
\fontsize{8.5}{10}\selectfont
    \begin{tabularx}{\linewidth}{c *{5}{C}} 
        \toprule
         & &   LIME  &   SHAP  &  IntGrad  &   Avg $\downarrow$ \\
        \midrule
    \multirow{ 3}{*}{Ins} & LeRF  &  5.2899 $\pm$ 1.4651   &  3.0199 $\pm$ 0.4789  &  1.5700 $\pm$ 0.6092  &  3.2933     \\
    & Insertion Test  &  1.3200  $\pm$ 0.4793  &  1.8999 $\pm$ 0.6451 &  3.4000 $\pm$ 0.6677  &   2.2066    \\
    & \textbf{\bise}   &  0.2599 $\pm$ 0.2848     &  0.05999  $\pm$ 0.0329   &  1.05999 $\pm$ 0.4175    &   0.4599      \\
    \midrule
    \multirow{ 3}{*}{Del} & MoRF  & 5.5000 $\pm$ 1.2597  &  4.6500 $\pm$ 1.2159 &  1.4600 $\pm$ 0.5149 &  3.8700    \\
    & Deletion Test  & 1.1299 $\pm$ 0.3970  &  2.7100 $\pm$ 0.4676  &  2.1700 $\pm$ 0.8380  &  2.0033      \\
    & \textbf{\bise}   &  0.9300 $\pm$ 0.2943   &  0.9100 $\pm$ 0.3997    &   1.4900  $\pm$ 0.7206  &  1.1100       \\   
        \bottomrule
    \end{tabularx}
    % \vskip{-0.1}
    \caption{Mean rank difference percentages with $\pm 1$ 
    SD across Swap perturbations (sz = 12) for insertion and deletion metrics; ImageNet-1K. }\label{tab:stddev_swap_imagenet}
\end{table}


\subsection{Certified Bounds Experiment}
\label{bounds_std}

% \input{icml2025/sections/figure_certified_bounds}
We calculate the certified upper and lower bounds across a range of $m$ (number of samples) and $\epsilon$ for $\delta=0.3$. These are computed for a LIME explanation using the insertion ordering. The average upper and lower bounds are plotted in Figure~\ref{epsilon_curves_fig}, and the average estimated value is plotted with a dotted line. The upper bounds are plotted with solid lines, while lower bounds are plotted with dashed lines. 

We see that, as $m$ increases, the bounds generally get closer to the estimated value. However, convergence of the bounds scales slowly with $m$ after $m$ is at least 3000, suggesting that a significantly larger sample size is needed to get very tight bounds. Nonetheless, a relatively small number of samples is sufficient to get within an order of magnitude. We note that for small $\epsilon$, the bound is not valid until $m$ is large enough, which is why not all $\epsilon$ curves can be extended to small $m$. We report the numerical values and the standard deviations for these curves in Table~\ref{tab:img_bd_std}, where the standard deviations are all below 0.1. 

% \paragraph{Standard deviations.} In Tables \ref{tab:img_bd_std} and 
% We fix $\delta = 0.3$. We use LIME insertion here.


\begin{table} 
    \begin{tabularx}{\linewidth}{c *{4}{C}}
        \toprule
        $\epsilon$ &  $m$ & \textbf{Lower Bound} & \textbf{Upper Bound}  \\
        \midrule
        0.1 & 5000 & 0.3262 $\pm$ 0.0207 & 0.7821 $\pm$ 0.0491 \\
        0.1 & 6000 & 0.3349 $\pm$ 0.0198 & 0.7381 $\pm$ 0.0427 \\
        0.1 & 9000 & 0.3525 $\pm$ 0.0170 & 0.6654 $\pm$ 0.0312 \\
        0.3  & 3000 & 0.3525 $\pm$ 0.0180 & 0.6753 $\pm$ 0.0329 \\
        0.3 & 5000 & 0.3719 $\pm$ 0.0284 & 0.6156 $\pm$ 0.0403 \\
        0.3 & 6000 & 0.3784 $\pm$ 0.0144 & 0.6004 $\pm$ 0.0206 \\
        0.3  & 9000 & 0.3912 $\pm$ 0.0261 & 0.5724 $\pm$ 0.034 \\
        0.5 & 1000 & 0.3266 $\pm$ 0.0230 & 0.8055 $\pm$ 0.0472\\
        0.5 &  3000 & 0.3722 $\pm$ 0.0219 & 0.6324 $\pm$ 0.0316 \\
        0.5 & 5000 & 0.3886 $\pm$ 0.0200 & 0.5940 $\pm$ 0.0227\\
        0.5  & 6000 & 0.3942 $\pm$ 0.0246 & 0.5840 $\pm$ 0.0283\\
        0.5  & 9000 & 0.4049 $\pm$ 0.0205 & 0.5651 $\pm$ 0.0224\\
        % 0.7 & 500 &  \\
        % 0.7  & 1000 &  \\
        % 0.7 & 3000 &  \\
        % 0.7 & 5000 &  \\
        % 0.7 & 6000 &  \\
        % 0.7 & 9000 &  \\
        % 0.9 & 500 &  \\
        % 0.9 & 1000 &  \\
        % 0.9  & 3000 &  \\
        % 0.9  & 5000 &  \\
        % 0.9 & 6000 &  \\
        % 0.9 & 9000 &  \\
        \bottomrule
    \end{tabularx}
    % \vskip{-0.1}
    \caption{Some examples of Insertion \bise \ bound estimation; ImageNet-1K} \label{tab:img_bd_std}
\end{table}



% \newpage
\section{Text Experiments}
\label{text_experiments}

\subsection{TweetEval Dataset Details}
Unlike the ImageNet-1K setting, where every image is the same size with the same number of features, TweetEval consists of tweets of varying length and therefore different number of features. Figure \ref{text_length} shows a histogram of tweet lengths in the TweetEval dataset. The majority of them lie in the 20-40 length range.

\begin{figure}
% \vskip 0.2in
\begin{center}
\includegraphics[width=0.7\columnwidth]{icml2025/images/text_length.png}
\caption{Histogram of Tweet Lengths in TweetEval dataset.}
\label{text_length}
\end{center}
\vskip -0.2in
\end{figure}

\subsection{Window and Swap Perturbations Experiment}
\paragraph{Insertion test and deletion test metrics are not robust to window perturbations. }Figure \ref{fig:insertionwindow_text} shows how the insertion test metric changes on average under window perturbations on the TweetEval dataset. Figure \ref{fig:deletionwindow_text} shows how the deletion test metric changes on average under window perturbations on the TweetEval dataset. Both the insertion test metric and the deletion test metric are not robust to these perturbations and can vary significantly when the ordering is perturbed by a small local window.


\paragraph{Insertion test and deletion test metrics are relatively better and less affected by swap perturbations. } Figure \ref{fig:insertionswap_text} shows how the insertion test metric changes on average under window perturbations on the TweetEval dataset. Figure \ref{fig:deletionswap_text} shows how the insertion test metric changes on average under window perturbations on the TweetEval dataset. 



\begin{figure}
% \vskip 0.2in
\begin{center}
\includegraphics[width=0.8\columnwidth]{icml2025/images/text_ordering_ins_bar_window.png}
\caption{Mean Insertion Test Metric under Window Perturbations; TweetEval.}
\label{fig:insertionwindow_text}
\end{center}
% \vskip -0.2in
\end{figure}

\begin{figure}
% \vskip 0.2in
\begin{center}
\includegraphics[width=0.8\columnwidth]{icml2025/images/text_ordering_del_bar_window.png}
\caption{Mean Deletion Test Metric under Window Perturbations; TweetEval.}
\label{fig:deletionwindow_text}
\end{center}
% \vskip -0.2in
\end{figure}

\begin{figure}
% \vskip 0.2in
\begin{center}
\includegraphics[width=0.8\columnwidth]{icml2025/images/text_ordering_ins_bar_swap.png}
\caption{Mean Insertion Test Metric under Swap Perturbations; TweetEval.}
\label{fig:insertionswap_text}
\end{center}
% \vskip -0.2in
\end{figure}

\begin{figure}
% \vskip 0.2in
\begin{center}
\includegraphics[width=0.8\columnwidth]{icml2025/images/text_ordering_del_bar_swap.png}
\caption{Mean Deletion Test Metric under Swap Perturbations; TweetEval.}
\label{fig:deletionswap_text}
\end{center}
% \vskip -0.2in
\end{figure}


\subsection{\bise Ordering Perturbations}
We repeat the same window and swap perturbations experiment but with the \bise metric. We find that across all perturbations, for both insertion and deletion modes, \bise stays relatively the same, which indicates that \bise is robust to these perturbations. Refer to Figures \ref{text_bise_1}, \ref{text_bise_2}, \ref{text_bise_3}, \ref{text_bise_4} for the average metric changes under these perturbations.

\begin{figure}
% \vskip 0.2in
\begin{center}
\includegraphics[width=0.8\columnwidth]{icml2025/images/text_ordering_bise_ins_bar_window.png}
\caption{Mean Insertion \bise Metric under Window Perturbations; TweetEval.}
\label{text_bise_1}
\end{center}
% \vskip -0.2in
\end{figure}

\begin{figure}
% \vskip 0.2in
\begin{center}
\includegraphics[width=0.8\columnwidth]{icml2025/images/text_ordering_bise_del_bar_window.png}
\caption{Mean Deletion \bise Metric under Window Perturbations; TweetEval.}
\label{text_bise_2}
\end{center}
% \vskip -0.2in
\end{figure}

\begin{figure}
% \vskip 0.2in
\begin{center}
\includegraphics[width=0.8\columnwidth]{icml2025/images/text_ordering_bise_ins_bar_swap.png}
\caption{Mean Insertion \bise Metric under Swap Perturbations; TweetEval.}
\label{text_bise_3}
\end{center}
% \vskip -0.2in
\end{figure}

\begin{figure}
% \vskip 0.2in
\begin{center}
\includegraphics[width=0.8\columnwidth]{icml2025/images/text_ordering_bise_del_bar_swap.png}
\caption{Mean Deletion \bise Metric under Swap Perturbations; TweetEval.}
\label{text_bise_4}
\end{center}
% \vskip -0.2in
\end{figure}




% \begin{figure}[ht]
% \vskip 0.2in
% \begin{center}
% \centerline{\includegraphics[width=1.2\columnwidth]{icml2025/figures/text_ordering_visualization.png}}
% \caption{Insertion and Deletion Accuracies of Text Perturbed Orderings}
% \label{}
% \end{center}
% \vskip -0.1in
% \end{figure}


\subsection{TweetEval Ranking Stability Experiment}

We perform the ranking stability experiment for TweetEval. Tables \ref{tab:stddev_window_text} and \ref{tab:stddev_swap_text} summarize the ranking stabilities of each setting, as well as the standard deviations. We report $\pm 1$ STD. For the most part, \bise is lower than all other metrics, which indicates it is more robust.

% \begin{table}
% \centering
% \small
% % \fontsize{8.5}{10}\selectfont
% \begin{tabular}{cccccccccc}
%     % \begin{tabularx}{\linewidth}{c *{5}{C} | c *{4}{C} }  %{ c *{8}{C} }
%         \toprule
%         &
%         & \multicolumn{4}{c}{Window}
%             & \multicolumn{4}{c}{Swap} \\
%         % \midrule
%         \cmidrule(lr){3-6} \cmidrule(lr){7-10}
    
%          & &   LIME  &   SHAP  &  IntGrad  &   Avg \downarrow &  LIME  &   SHAP  &   IntGrad  &   Avg \downarrow \\
%         \midrule
%     \multirow{ 3}{*}{Ins} & LeRF  &  52.9352    & 90.0689   &  90.0689  &  77.691  & 26.2491  &  38.5151   &   33.2610  &  32.6750  \\
%     & Ins. Test & 96.5094    & 164.6417   & 164.6417 & 141.9309 &  43.1484  &  64.7860   &  56.0703   &   54.6682      \\
%     % & Max-Sensitivity   &     &     &    &     &    &     &    &     \\
%     % & Infidelity   &     &     &    &     &    &     &    &     \\
%     % Fidelity   &     &     &    &     &    &     &    &     \\
%     % Stability   &     &     &    &     &    &     &    &     \\
%     % Comp   &       &       &       &       &       &       &       &       \\
%     & \textbf{Ins. \bise}   &   36.5277    &   31.8128   &   30.9704    &   33.1036   &  36.0661      &  27.1076    &  35.1717     &   32.7818   \\
%     % & \textbf{\bise\ Upper Bd}   &    &  &  & & &   \\
%     \midrule
    
%     \multirow{ 3}{*}{Del} & MoRF  &  34.8078   &  70.8282  &  70.8282   & 58.8214  & 20.9085   &  32.1372   &  39.1491  &  30.7316   \\
%     & Del. Test  &  79.4447   &  116.9021   & 116.9021  & 104.4163 & 43.5151 & 58.0302 &  63.2941 & 54.9464  \\
%     % LeRF   &     &     &    &     &    &     &    &     \\
%     % & Max Sensitivity   &     &     &    &     &    &     &    &     \\
%     % & Infidelity   &     &     &    &     &    &     &    &     \\
%     % Fidelity   &     &     &    &     &    &     &    &     \\
%     % Stability   &     &     &    &     &    &     &    &     \\
%     % Comp   &       &       &       &       &       &       &       &       \\
%     & \textbf{Del. \bise}   &   37.1956   &  24.1505   &  21.8698    &  27.7386    &  35.5777     &  31.7213    &  26.6347    &  31.3112    \\
%     % & \textbf{\bise\ Upper Bd}   &      \\
%         \bottomrule
%     \end{tabular}
%     % \end{tabularx}
%     % \caption{Mean Rank Differences Across Insertion Metrics and Perturbations (sz = 12); ImageNet-1K. Bolded indicates the lowest mean rank difference. }\label{tab:1}\\
%     \caption{Mean rank differences across perturbations (sz = 4) for insertion and deletion metrics; TweetEval. }\label{tab:2}
% \end{table} \label{tab:rank_diff_text}
    % Bolded indicates the lowest mean rank difference


    

% \begin{tabularx}{\linewidth}{c *{4}{C} | c *{4}{C} }
%     \toprule
%     & \multicolumn{4}{c |}{Sliding Window}
%         & \multicolumn{4}{c}{Features Moved} \\
%     % \midrule
%     \cmidrule(lr){2-5} \cmidrule(lr){6-10}

%      &   LIME  &   SHAP  &  IntGrad  &   Avg  &  LIME  &   SHAP  &   IntGrad  &   Avg  \\
%     \midrule
% LeRF  &     &     &     &     &     &     &     &     \\
% Classic Acc  &     &     &     &     &     &     &     &     \\
% % LeRF   &     &     &    &     &    &     &    &     \\
% Max Sensitivity   &     &     &    &     &    &     &    &     \\
% Infidelity   &     &     &    &     &    &     &    &     \\
% Fidelity   &     &     &    &     &    &     &    &     \\
% Stability   &     &     &    &     &    &     &    &     \\
% % Comp   &       &       &       &       &       &       &       &       \\
% \textbf{Influence}   &       &       &       &       &       &       &       &       \\
% % \textbf{Influence Upper Bound}  &       &       &       &       &       &       &       &       \\
%     \bottomrule
% \caption{Mean Rank Differences Across Insertion Metrics and Perturbations; TweetEval}\label{tab:4}\\
% \end{tabularx}

% \begin{tabularx}{\linewidth}{c *{4}{C} | c *{4}{C} }
%     \toprule
%     & \multicolumn{4}{c |}{Sliding Window}
%         & \multicolumn{4}{c}{Features Moved} \\
%     % \midrule
%     \cmidrule(lr){2-5} \cmidrule(lr){6-10}

%      &   LIME  &   SHAP  &  IntGrad  &   Avg  &  LIME  &   SHAP  &   IntGrad  &   Avg  \\
%     \midrule
% MoRF  &     &     &     &     &     &     &     &     \\
% Classic Acc  &     &     &     &     &     &     &     &     \\
% % LeRF   &     &     &    &     &    &     &    &     \\
% Max Sensitivity   &     &     &    &     &    &     &    &     \\
% Infidelity   &     &     &    &     &    &     &    &     \\
% Fidelity   &     &     &    &     &    &     &    &     \\
% Stability   &     &     &    &     &    &     &    &     \\
% % Comp   &       &       &       &       &       &       &       &       \\
% \textbf{Influence}   &       &       &       &       &       &       &       &       \\
% % \textbf{Influence Upper Bound}  &       &       &       &       &       &       &       &       \\
%     \bottomrule
% \caption{Mean Rank Differences Across Deletion Metrics and Perturbations; TweetEval}\label{tab:5}\\
% \end{tabularx}




\begin{table}
\centering
\fontsize{8.5}{10}\selectfont
    \begin{tabularx}{\linewidth}{c *{5}{C}}  
        \toprule
         & &   LIME  &   SHAP  &  IntGrad  &   Avg $\downarrow$ \\
        \midrule
    \multirow{ 3}{*}{Ins} & LeRF  &  52.9352 $\pm$ 2.5729 & 90.0689 $\pm$ 7.4862 & 90.0689 $\pm$ 5.6761 & 77.691   \\
    & Ins. Test  &  96.5094 $\pm$ 4.6539 & 164.6417 $\pm$ 9.6535 & 164.6417 $\pm$ 7.2451 & 141.9309   \\
    & \textbf{\bise}   &   36.5277 $\pm$ 5.2660 & 31.8128 $\pm$ 3.6497 & 30.9704 $\pm$ 3.5152 & 33.1036      \\
    \midrule
    \multirow{ 3}{*}{Del} & MoRF  &   34.8078 $\pm$ 1.9437 & 70.8282 $\pm$ 3.3531 & 70.8282 $\pm$ 4.9471 & 58.8214  \\
    & Del. Test  &    79.4447 $\pm$ 3.6656 & 116.9021 $\pm$ 9.0746 & 116.9021 $\pm$ 7.8079 & 104.4163   \\
    & \textbf{\bise}   &    37.1956 $\pm$ 4.3674 &  24.1505 $\pm$ 1.2221 & 21.8698 $\pm$ 4.4695 & 27.7386    \\
        \bottomrule
    \end{tabularx}

    \caption{Mean rank differences with $\pm 1$ standard deviation across Window perturbations (sz = 12) for insertion and deletion metrics; TweetEval. }\label{tab:stddev_window_text}
\end{table}


  



\begin{table}
\centering
\fontsize{8.5}{10}\selectfont
    \begin{tabularx}{\linewidth}{c *{5}{C}} 
        \toprule
         & &   LIME  &   SHAP  &  IntGrad  &   Avg $\downarrow$ \\
        \midrule
    \multirow{ 3}{*}{Ins} & LeRF & 26.2491 $\pm$ 3.2782 & 38.5151 $\pm$ 4.8620 & 33.2610 $\pm$ 3.6936 & 32.6750 \\
    & Ins. Test  & 43.1484 $\pm$ 5.9566 & 64.7860 $\pm$ 3.1062 & 56.0703 $\pm$ 4.4236 & 54.6682 \\
    & \textbf{\bise} & 36.0661 $\pm$ 5.3840 & 27.1076 $\pm$ 1.5597 & 35.1717 $\pm$ 4.0249 & 32.7818 \\
    \multirow{ 3}{*}{Del} & MoRF & 20.9085 $\pm$ 1.9958 & 32.1372 $\pm$ 4.3084 & 39.1491 $\pm$ 4.7868  & 30.7316 \\
    & Del. Test  & 43.5151 $\pm$ 4.4850 & 58.0302 $\pm$ 7.1649 & 63.2941 $\pm$ 3.8872 & 54.9464 \\
    & \textbf{\bise} & 35.5777 $\pm$ 4.5628 &  31.7213 $\pm$  3.1655 & 26.6347 $\pm$ 2.5774 & 31.3112 \\
   
        \bottomrule
    \end{tabularx}

    \caption{Mean rank differences with $\pm 1$ standard deviation across Swap perturbations (sz = 4) for insertion and deletion metrics; TweetEval. }\label{tab:stddev_swap_text}
\end{table}

\subsection{Certified Bounds Experiment}
We fix $\delta = 0.3$. We use LIME insertion here. 


\begin{figure} 
% \vskip 0.2in
\begin{center}
\includegraphics[width=0.7\columnwidth]{icml2025/images/eps_curves_text.png}
\caption{We plot a curve for each $\epsilon$. A curve comprises of the mean (upper or lower) bound across all TweetEval examples for increasing $m$, the number of samples for each influence calculation. The mean of \bise estimates across examples is denoted by the black dotted line. We fix $\delta = 0.3$.}
\label{epsilon_curves_fig}
\end{center}
% \vskip -0.2in
\end{figure}


\begin{table}
\centering
\small
    \begin{tabular}{cccc}
        \toprule
        $\epsilon$ &  $m$ & \textbf{Lower Bound} & \textbf{Upper Bound}  \\
        \midrule
        0.5 & 1000 & 0.1230 $\pm$ 0.0027 & 0.3547 $\pm$ 0.0053\\
        0.5 &  5000 & 0.1466 $\pm$ 0.0219 & 0.2947 $\pm$ 0.0316 \\
        0.7 & 500 & 0.1165 $\pm$ 0.0027 & 0.4420 $\pm$ 0.0050 \\
        0.7  & 1000 & 0.1288 $\pm$ 0.0021 & 0.3933 $\pm$ 0.0022 \\
        0.7 & 5000 & 0.1502 $\pm$ 0.0041 & 0.3647 $\pm$ 0.0015 \\
        0.9  & 500 & 0.1212 $\pm$ 0.0010 & 0.4871 $\pm$ 0.0018 \\
        0.9 & 1000 & 0.1329 $\pm$ 0.0018 & 0.4641 $\pm$ 0.0009 \\
        0.9 & 5000 & 0.1526 $\pm$ 0.0020 & 0.4530 $\pm$ 0.0004 \\
        \bottomrule
    \end{tabular}
    \caption{Some examples of Insertion \bise \ bound estimation; TweetEval.}
\end{table} \label{tab:text_bd_std}


\section{Additional Experiments}

\subsection{Finding optimal $m$ for \bise metric}
$m$ represents the number of samples the \bise metric takes for each approximate influence calculation at each $k$. We tested for $m = [1, 50, 100, 300, 500, 1000, 5000, 9000] $. For each $m$, we calculated scores and took the mean of those samples five times, and report the variance of the means in Figure \ref{m_variance}. For the text version, see Figure \ref{m_variance_text}. For ImageNet-1K experiments involving all examples, we mainly took $m = 50$ (and $m = 300$). And for TweetEval experimetns involving all examples, we took $m = 100$.

\begin{figure}[ht!]
\vskip 0.2in
\begin{center}
\includegraphics[width=0.5\columnwidth]{icml2025/images/imagenet_m_variance.png}
\caption{Variance of sample means (\# of samples = 5) for different $m$,  ImageNet1K.}
\label{m_variance}
\end{center}
\vskip -0.2in
\end{figure}


\begin{figure}[ht!]
\vskip 0.2in
\begin{center}
\includegraphics[width=0.5\columnwidth]{icml2025/images/text_m_variance.png}
\caption{Variance of sample means (\# of samples = 5) for different $m$, TweetEval.}
\label{m_variance_text}
\end{center}
\vskip -0.2in
\end{figure}

\subsection{Varying step size for metric calculation}
In the simplest case, we use step size = 1. For the majority of our experiments, we used step size = 4 for faster computation.

\newpage

\section{Prior Reviews}
We show below reviews of the last submission of this paper. From their feedback, we have addressed the following:
\begin{itemize}
    \item We have expanded on and justified the premise of the work – that attribution methods should be robust to ordering perturbations in the introduction. We also added a human evaluation study to see what practitioners would expect from a good and robust explanation evaluation metric. Our results match our intuition, that small perturbations should result in small changes in scores, but larger perturbations should result in larger changes in scores.
    \item Regarding the existing works investigating the reliability of deletion and insertion metrics that was brought up in previous reviews (such as benchmarks such as ROAR, ROAD and CLEVR-XAI), we have taken them into account and categorized them according to where they are situated in relation to our work. 
    \item We have also clarified specific properties that metrics for evaluating explanation methods should possess to be trustworthy.
    \item To avoid confusion and misunderstanding, we have renamed our certified bounds to be a corollary (versus a lemma) from the original theorem presented in \citep{levi2020tolerant}. Our contribution is the application of the boolean function theory result to evaluating explanation methods.
    \item We have expanded our discussion on sample complexity.
\end{itemize}


% “The premise of the work – that attribution methods should be robust to ordering perturbations – is asserted without justification. There is no argument in the paper about why being robust to ordering perturbations is desirable.” “There is no qualitative analysis showing the circumstances in which BISE should be preferred (or dispreferred) to other metrics. “ (U8TA). This motivation was also questioned by reviewer 7CK5.
% “Existing works have extensively investigated the unreliability of deletion and insertion metrics. To address these issues, benchmarks such as ROAR [1], ROAD [2], DiFull, and CLEVR-XAI [3] have already been proposed for attribution evaluation.” (7CK5)
% Triviality of theoretical results. “The influence estimation bounds are a direct consequence of Levi [2020]” (Tq2D); “The probabilistic correctness of the approximation is a direct consequence of existing results in Boolean set influence. This should be made clearer in the abstract and the introduction.” (aEcC)
% limited experiments make it “unclear if the proposed approach would work in practice”. “The experimental evaluation is significantly lacking” (Tq2D). “The evaluation in the paper is limited.” (7CK5)
% Sample complexity
