# Supplementary material for: Probabilistic Stability Guarantees for Feature Attributions
Source: arXiv:2504.13787 source file (2025-08-07)
Supplement: Supplementary file 2 [file roberta_soft_vs_hard_stability_appendix.tex]

\begin{figure*}[t]
\centering
\begin{minipage}{0.31\textwidth}
    \centering
    \includegraphics[width=\linewidth]{images/roberta_imagenet_softvhard_lime.pdf}
\end{minipage}
\quad
\begin{minipage}{0.31\textwidth}
    \centering
    \includegraphics[width=\linewidth]{images/roberta_imagenet_softvhard_shap.pdf}
\end{minipage}
\quad
\begin{minipage}{0.31\textwidth}
    \centering
    \includegraphics[width=\linewidth]{images/roberta_imagenet_softvhard_intgrad.pdf}
\end{minipage}


\begin{minipage}{0.31\textwidth}
    \centering
    \includegraphics[width=\linewidth]{images/roberta_imagenet_softvhard_mfaba.pdf}
\end{minipage}
\quad
\begin{minipage}{0.31\textwidth}
    \centering
    \includegraphics[width=\linewidth]{images/roberta_imagenet_softvhard_random.pdf}
\end{minipage}

\caption{
\textbf{(RoBERTa) There is a large gap between the soft and hard stability rates.}
}
\label{fig:roberta_soft_vs_hard_stability_appendix}
\end{figure*}
